# Supplementary material for: UP: Unbounded Positive Asymmetric Optimization for Breaking the Exploration-Stability Dilemma
Source: arXiv:2607.06987 source file (2026-07-08)
Supplement: Supplementary file 1 [file gradient_bias.tex]

\section{Theoretical Analysis of Gradient Bias}
\label{sec:theoretical_analysis}

In this section, we rigorously quantify the theoretical gradient bias introduced by the proposed UP method compared to the standard clipped Group Relative Policy Optimization (GRPO). We first establish the on-policy REINFORCE gradient as an unbiased ground truth, then derive closed-form expressions for the bias of both UP and GRPO, and finally contrast these bias expressions at the level of their integrands. The key conclusion is that, as the current policy drifts from the behavior policy, UP's bias is a vanishing perturbation while GRPO's bias contains a persistent, irreducible contribution from clipped samples---and this contribution concentrates precisely on the exploration-critical long-tail tokens identified in Sec.~3.3.

\subsection{Preliminaries and the On-Policy REINFORCE Baseline}

In the context of Large Language Model (LLM) reasoning, the generation process can be formulated as a Contextual Bandit problem. The state $s$ (i.e., the prompt) is drawn from a fixed dataset distribution $P(s)$, independent of any prior actions. The action $a$ (i.e., the complete sequence of generated tokens) is sampled from the current policy $\pi_\theta(a|s)$. Let $R(s, a)$ denote the exact absolute reward provided by the environment or a reward model.

The objective of the true on-policy REINFORCE algorithm is to maximize the expected reward. Applying the log-derivative trick ($\nabla_\theta \pi_\theta(a|s) = \pi_\theta(a|s) \nabla_\theta \log \pi_\theta(a|s)$), the exact on-policy expected gradient $g_{\text{REINFORCE\_on}}$ is:
\begin{equation} \label{eq:g_reinforce_on_raw}
    g_{\text{REINFORCE\_on}} = \mathbb{E}_{s \sim P,\, a \sim \pi_\theta} \left[ \nabla_\theta \log \pi_\theta(a|s) \, R(s,a) \right]
\end{equation}

To reduce the high variance of the Monte Carlo gradient estimator, it is standard practice to introduce a state-dependent baseline $b(s)$ (such as the group-mean reward in GRPO). A fundamental property of the score function estimator is that subtracting any baseline independent of action $a$ does not alter the expected gradient: $\mathbb{E}_{a \sim \pi_\theta}[\nabla_\theta \log \pi_\theta(a|s) b(s)] = b(s) \nabla_\theta \sum_a \pi_\theta(a|s) = 0$.

Defining the advantage as $A_{\text{old}}(s, a) = R(s, a) - b(s)$, we rewrite Eq.~\ref{eq:g_reinforce_on_raw} without introducing any bias:
\begin{equation} \label{eq:g_reinforce_on_advantage}
    g_{\text{REINFORCE\_on}} = \mathbb{E}_{s \sim P,\, a \sim \pi_\theta} \left[ \nabla_\theta \log \pi_\theta(a|s) \, A_{\text{old}}(s,a) \right]
\end{equation}

\textit{Remark on group-relative advantages.} For the group-mean baseline used in GRPO/DAPO, the unbiasedness above is exact. The std-normalization factor introduces only an action-dependent positive scaling that preserves the gradient direction; we therefore treat it as an $O(1)$ reweighting throughout this analysis and omit it from the notation for clarity.

Since off-policy algorithms like PPO and GRPO perform multiple optimization epochs using data collected by an older behavior policy $\pi_{\text{old}}$, we apply Importance Sampling (IS) to Eq.~\ref{eq:g_reinforce_on_advantage} to establish a baseline that shares the same sampling distribution. Multiplying and dividing by $\pi_{\text{old}}(a|s)$:
\begin{equation} \label{eq:g_reinforce_on_is}
    g_{\text{REINFORCE\_on}} = \mathbb{E}_{s \sim P,\, a \sim \pi_{\text{old}}} \left[ \frac{\pi_\theta(a|s)}{\pi_{\text{old}}(a|s)} \nabla_\theta \log \pi_\theta(a|s) \, A_{\text{old}}(s,a) \right]
\end{equation}

Equation~\ref{eq:g_reinforce_on_is} serves as our absolute ground truth for an unbiased gradient expectation under experience replay. All subsequent bias analyses are defined as deviations from this reference.

\subsection{Gradient Bias of the Proposed UP ($\text{Bias}_{\text{UP}}$)}

We first establish that the stop-gradient construction in UP yields a surrogate whose expected gradient admits a clean closed form. Because $\operatorname{sg}(\pi_\theta(a|s))$ is a constant with respect to $\theta$ whose forward value equals $\pi_\theta(a|s)$, the surrogate $\pi_\theta / \operatorname{sg}(\pi_\theta)$ produces, upon differentiation:
\begin{equation}
    \nabla_\theta \left[ \frac{\pi_\theta(a|s)}{\operatorname{sg}(\pi_\theta(a|s))} \right] = \frac{\nabla_\theta \pi_\theta(a|s)}{\pi_\theta(a|s)} = \nabla_\theta \log \pi_\theta(a|s)
\end{equation}

Thus, for positive advantage samples ($A_{\text{old}} > 0$), UP intentionally discards the importance sampling weight, yielding a self-anchored surrogate whose expected gradient coincides with off-policy advantage-weighted log-likelihood maximization:
\begin{equation} \label{eq:g_up}
    g_{\text{UP}} = \mathbb{E}_{s \sim P,\, a \sim \pi_{\text{old}}} \left[ \nabla_\theta \log \pi_\theta(a|s) \, A_{\text{old}}(s,a) \right]
\end{equation}

Note the crucial distinction from Eq.~\ref{eq:g_reinforce_on_advantage}: although $g_{\text{UP}}$ shares the same integrand structure as the on-policy REINFORCE gradient, the expectation is taken over $\pi_{\text{old}}$ rather than $\pi_\theta$. Consequently, when $\pi_\theta \neq \pi_{\text{old}}$, $g_{\text{UP}}$ is no longer an unbiased estimate of $g_{\text{REINFORCE\_on}}$.

We define the gradient bias of UP ($\text{Bias}_{\text{UP}}$) as the difference between its expected surrogate gradient and the on-policy ground truth. Subtracting Eq.~\ref{eq:g_reinforce_on_is} from Eq.~\ref{eq:g_up}:
\begin{align}
    \text{Bias}_{\text{UP}} &= g_{\text{UP}} - g_{\text{REINFORCE\_on}} \nonumber \\
    &= \mathbb{E}_{s \sim P,\, a \sim \pi_{\text{old}}} \left[ \left(1 - \frac{\pi_\theta(a|s)}{\pi_{\text{old}}(a|s)}\right) \nabla_\theta \log \pi_\theta(a|s) \, A_{\text{old}}(s,a) \right] \label{eq:bias_up}
\end{align}

\textbf{Remark (Nature of $\text{Bias}_{\text{UP}}$).} Equation~\ref{eq:bias_up} demonstrates that UP introduces a systematic, \textit{first-order bias} whose integrand is
\begin{equation} \label{eq:bias_up_integrand}
    \mathcal{I}_{\text{UP}}(s, a; \theta) \;=\; \left(1 - \frac{\pi_\theta(a|s)}{\pi_{\text{old}}(a|s)}\right) \nabla_\theta \log \pi_\theta(a|s) \, A_{\text{old}}(s,a).
\end{equation}
The magnitude and direction of this bias are directly governed by the policy divergence factor $(1 - \pi_\theta/\pi_{\text{old}})$: as the current policy deviates from the rollout policy, the uncorrected discrepancy grows; conversely, as $\pi_\theta \to \pi_{\text{old}}$, this factor smoothly vanishes and so does the entire bias integrand. The bias is \textit{global} in support (it affects all samples) but \textit{vanishes pointwise} in the small-drift regime. We will return to this vanishing property when comparing against GRPO in Sec.~\ref{subsec:bias_comparison}.

\subsection{Gradient Bias of the Clipped GRPO ($\text{Bias}_{\text{GRPO}}$)}

Let the importance sampling ratio be $r_t(\theta) = \pi_\theta(a|s) / \pi_{\text{old}}(a|s)$. The standard clipped GRPO objective is:
\begin{equation}
    L^{\text{GRPO}}(\theta) = \mathbb{E}_{s \sim P,\, a \sim \pi_{\text{old}}} \left[ \min\Big(r_t(\theta) A_{\text{old}},\; \operatorname{clip}\big(r_t(\theta), 1-\epsilon, 1+\epsilon\big) A_{\text{old}}\Big) \right]
\end{equation}

The clipping mechanism introduces non-linearity. To compute the expected gradient, we partition the sampled action space into two mutually exclusive sets based on whether the clipping constraint is active:
\begin{itemize}
    \item \textbf{Unclipped Region $\mathcal{U}$:} The ratio $r_t(\theta)$ is within $[1-\epsilon, 1+\epsilon]$, or the advantage sign makes the clip inactive. Here, the local objective is $r_t(\theta) A_{\text{old}}$.
    \item \textbf{Clipped Region $\mathcal{C}$:} The clip is active. The local objective becomes $(1 \pm \epsilon) A_{\text{old}}$. Since $\epsilon$ and $A_{\text{old}}$ are constants with respect to $\theta$, the gradient in this region is exactly $\mathbf{0}$.
\end{itemize}

Let $\mathbb{I}_{\mathcal{U}}$ and $\mathbb{I}_{\mathcal{C}}$ be indicator functions for these regions, satisfying $\mathbb{I}_{\mathcal{U}} + \mathbb{I}_{\mathcal{C}} = 1$. Using $\nabla_\theta r_t(\theta) = r_t(\theta) \nabla_\theta \log \pi_\theta(a|s)$, the expected gradient of clipped GRPO is:
\begin{align} \label{eq:g_grpo_clip}
    g_{\text{GRPO\_clip}} &= \nabla_\theta L^{\text{GRPO}}(\theta) \nonumber \\
    &= \mathbb{E}_{\pi_{\text{old}}} \left[ \mathbb{I}_{\mathcal{U}} \cdot \nabla_\theta \big(r_t(\theta) A_{\text{old}}\big) + \mathbb{I}_{\mathcal{C}} \cdot \mathbf{0} \right] \nonumber \\
    &= \mathbb{E}_{\pi_{\text{old}}} \left[ \mathbb{I}_{\mathcal{U}} \cdot \frac{\pi_\theta(a|s)}{\pi_{\text{old}}(a|s)} \nabla_\theta \log \pi_\theta(a|s) \, A_{\text{old}}(s,a) \right]
\end{align}

To compute the exact bias, we partition the unbiased on-policy baseline Eq.~\ref{eq:g_reinforce_on_is} using the same indicators: $g_{\text{REINFORCE\_on}} = \mathbb{E}_{\pi_{\text{old}}}\big[(\mathbb{I}_{\mathcal{U}} + \mathbb{I}_{\mathcal{C}}) \cdot r_t(\theta) \nabla_\theta \log \pi_\theta \, A_{\text{old}}\big]$. Subtracting this from Eq.~\ref{eq:g_grpo_clip}, the unclipped-region terms cancel exactly, leaving:
\begin{align} \label{eq:bias_grpo}
    \text{Bias}_{\text{GRPO}} &= g_{\text{GRPO\_clip}} - g_{\text{REINFORCE\_on}} \nonumber \\
    &= -\, \mathbb{E}_{\pi_{\text{old}}} \left[ \mathbb{I}_{\mathcal{C}} \cdot \frac{\pi_\theta(a|s)}{\pi_{\text{old}}(a|s)} \nabla_\theta \log \pi_\theta(a|s) \, A_{\text{old}}(s,a) \right]
\end{align}

\textbf{Remark (Nature of $\text{Bias}_{\text{GRPO}}$).} Equation~\ref{eq:bias_grpo} confirms that standard GRPO also exhibits bias, with integrand
\begin{equation} \label{eq:bias_grpo_integrand}
    \mathcal{I}_{\text{GRPO}}(s, a; \theta) \;=\; -\,\mathbb{I}_{\mathcal{C}}(s, a) \cdot r_t(\theta) \cdot \nabla_\theta \log \pi_\theta(a|s) \, A_{\text{old}}(s, a).
\end{equation}
The structure of this integrand is fundamentally different from Eq.~\ref{eq:bias_up_integrand}. The strict dependence on $\mathbb{I}_{\mathcal{C}}$ means GRPO's bias is a \textit{support-restricted} bias: it contributes only on the clipped region $\mathcal{C}$, where it \textit{subtracts} the gradient mass of samples that violate the trust region. This yields the familiar approximate trust-region improvement guarantee of PPO-style methods~\citep{schulman2015trust, schulman2017proximal}. However, the clipped region $\mathcal{C}$ under positive advantages is populated disproportionately by the \textbf{low-$\pi_{\text{old}}$ correct-reasoning tokens} whose probability ratio inflates rapidly as $\pi_\theta$ improves---exactly the long-tail trajectories identified in Sec.~3.3 as the bottleneck of reasoning exploration.

\subsection{Extension to UP-DAPO and UP-GSPO}

The preceding analysis extends naturally to the other UP variants instantiated in the main text.

\textbf{UP-DAPO (token-level).} Replacing the sequence-level action $a$ with a token $o_{i,t}$ and the advantage $A_{\text{old}}$ with the token-level DAPO advantage $\hat{A}_{i,t}$ yields identical bias expressions (Eqs.~\ref{eq:bias_up}, \ref{eq:bias_grpo}) under the token-level importance ratio $r_{i,t}(\theta)$.

\textbf{UP-GSPO (sequence-level).} For the length-normalized sequence-level ratio $s_i(\theta) = (\pi_\theta(o_i|q)/\pi_{\text{old}}(o_i|q))^{1/|o_i|}$, the positive-branch UP-GSPO surrogate yields (by Appendix~C) a length-normalized REINFORCE gradient. The corresponding bias becomes:
\begin{equation}
    \text{Bias}_{\text{UP-GSPO}} = \mathbb{E}_{\pi_{\text{old}}}\!\left[\big(1 - s_i(\theta)\big) \cdot \frac{1}{|o_i|} \sum_{t=1}^{|o_i|} \nabla_\theta \log \pi_\theta(o_{i,t}|q, o_{i,<t}) \cdot \hat{A}_i\right]
\end{equation}
The same pointwise-vanishing structure holds: as $s_i(\theta) \to 1$, the entire integrand vanishes.

\textbf{Negative branch.} For $\hat{A} \leq 0$, UP retains the standard clipped objective; the negative branch therefore inherits exactly $\text{Bias}_{\text{GRPO}}$ (Eq.~\ref{eq:bias_grpo}). The overall UP bias is a mixture: a pointwise-vanishing first-order bias on positive samples, and a support-restricted bias on negative samples---consistent with the asymmetric design motivation in Sec.~4.

\subsection{Comparative Analysis: Vanishing vs.\ Persistent Bias Integrands}
\label{subsec:bias_comparison}

We now compare the two bias expressions directly, at the level of their integrands (Eqs.~\ref{eq:bias_up_integrand}, \ref{eq:bias_grpo_integrand}), rather than their upper bounds. This integrand-level comparison is sharper and more robust than a bound-level comparison: an upper bound is a loose summary that can shift with the choice of factorization, whereas the integrand is an intrinsic property of the bias itself.

\paragraph{(i) UP's bias integrand vanishes in the small-drift limit.} By Eq.~\ref{eq:bias_up_integrand}, the UP bias integrand factors as
\begin{equation}
    \mathcal{I}_{\text{UP}}(s, a; \theta) \;=\; \underbrace{\big(1 - r_t(\theta)\big)}_{\text{vanishing factor}} \cdot \underbrace{\nabla_\theta \log \pi_\theta(a|s) \, A_{\text{old}}(s, a)}_{\text{on-policy REINFORCE integrand}}.
\end{equation}
The second factor is precisely the on-policy REINFORCE integrand---bounded in expectation by the reward landscape and policy parameterization. The first factor, $(1 - r_t(\theta))$, is a pointwise measure of policy drift that vanishes smoothly as $\pi_\theta \to \pi_{\text{old}}$. Crucially, this vanishing occurs \textit{pointwise at every sample}, not just in expectation: every term in the bias integral is individually suppressed as the policy drift shrinks. In our training regime, where the measured KL stays near $10^{-3}$ throughout training (Fig.~4), $|1 - r_t(\theta)|$ is uniformly small across samples, rendering UP's bias a \textit{vanishing perturbation} on the on-policy gradient.

\paragraph{(ii) GRPO's bias integrand contains a persistent, non-vanishing contribution.} By Eq.~\ref{eq:bias_grpo_integrand}, the GRPO bias integrand is
\begin{equation}
    \mathcal{I}_{\text{GRPO}}(s, a; \theta) \;=\; -\,\mathbb{I}_{\mathcal{C}}(s, a) \cdot r_t(\theta) \cdot \nabla_\theta \log \pi_\theta(a|s) \, A_{\text{old}}(s, a).
\end{equation}
On the clipped region $\mathcal{C}$, by definition $r_t(\theta) \geq 1 + \epsilon$ (or $r_t(\theta) \leq 1 - \epsilon$). The integrand therefore does \textit{not} vanish pointwise as the policy drift shrinks: whenever a sample falls into $\mathcal{C}$, its contribution to the bias is at least $(1 + \epsilon)$ times the on-policy integrand, regardless of how small the overall drift is. The bias vanishes only in the \textit{global} sense of $p_{\mathcal{C}}(\theta) \to 0$, i.e., when no sample triggers clipping at all. As long as \textit{any} sample falls into $\mathcal{C}$---and empirically some always do---the GRPO bias contains an irreducible, finite-magnitude contribution from each such sample.

\paragraph{(iii) The structural asymmetry is decisive.} The two integrands exhibit fundamentally different limiting behavior as the policy evolves:
\begin{center}
\begin{tabular}{ll}
\toprule
UP: & $\mathcal{I}_{\text{UP}} \to 0$ pointwise as $r_t(\theta) \to 1$. \\
GRPO: & $\mathcal{I}_{\text{GRPO}}$ retains finite mass on $\mathcal{C}$ regardless of overall drift. \\
\bottomrule
\end{tabular}
\end{center}
This asymmetry is the decisive structural difference between the two methods. UP's bias scales with policy drift and can be made arbitrarily small by controlling drift (e.g., via learning rate and mini-batch count); GRPO's bias cannot be analogously controlled, because it is triggered not by the global drift but by individual samples crossing the clip boundary---samples that, by the Probability Capacity analysis in Sec.~3.3, are precisely the low-$\pi_{\text{old}}$ correct-reasoning tokens.

\paragraph{(iv) Alignment with exploration.} The structural asymmetry above aligns directly with the exploration objective. UP's vanishing bias preserves the gradient signal of every sample, including the low-$\pi_{\text{old}}$ correct-reasoning tokens whose reinforcement is essential for discovering rare reasoning trajectories. GRPO's persistent bias, in contrast, is concentrated on exactly these samples: it zeroes out their gradient (Eq.~\ref{eq:g_grpo_clip}) and leaves a residual bias term (Eq.~\ref{eq:bias_grpo}) that cannot be suppressed by reducing drift. In the bias--exploration trade-off, UP's integrand is \textit{structurally compatible} with exploration (bias vanishes where it would otherwise interfere), while GRPO's integrand is \textit{structurally opposed} to exploration (bias persists precisely on the samples exploration depends on).

\paragraph{Empirical verification.} Figs.~3(a) and 3(b) provide direct evidence for this structural argument. UP-DAPO exhibits substantially higher generation entropy and a higher Best@32 ceiling on AIME24 than DAPO, despite both methods maintaining low KL divergence throughout training (Fig.~4). The higher exploration capacity of UP cannot be explained by UP having a smaller total bias---our analysis makes no such claim. Rather, it arises from UP's bias being a vanishing perturbation that spares exploration-critical samples, while GRPO's bias persists on exactly those samples and truncates their gradient contribution entirely.

\paragraph{Summary.} Equations~\ref{eq:bias_up_integrand} and~\ref{eq:bias_grpo_integrand} give the exact, closed-form bias integrands of UP and GRPO. The comparison is structural: UP's integrand vanishes pointwise in the small-drift regime, while GRPO's integrand retains an irreducible contribution from the clipped region that does not vanish with shrinking drift. Because the clipped region coincides with the exploration-critical long-tail tokens (Sec.~3.3), GRPO's bias is structurally opposed to exploration, whereas UP's bias is structurally compatible with it. This integrand-level analysis completes the theoretical justification for UP: \textit{UP's advantage over GRPO is not about carrying less bias, but about carrying a bias that vanishes where exploration needs gradient signal, rather than persisting where exploration is most fragile}.
